# Supplementary material for: Management Decisions in Manufacturing using Causal Machine Learning -- To Rework, or not to Rework?
Source: arXiv:2406.11308 source file (2024-06-17)
Supplement: Supplementary file 1 [file results_L4.tex]

\section{Results for Product Type ``T2''}
\label{app:L4}
In this Section, we will present the analysis for product type ``T2''. Overall, the results are very similar, as the process is the same but only the product properties differ to some extend. Also in this setting, we would suggest a cut-off along the main component.
\subsection{Results}
\begin{figure}[ht]
    \centering
    \includegraphics[width=\linewidth]{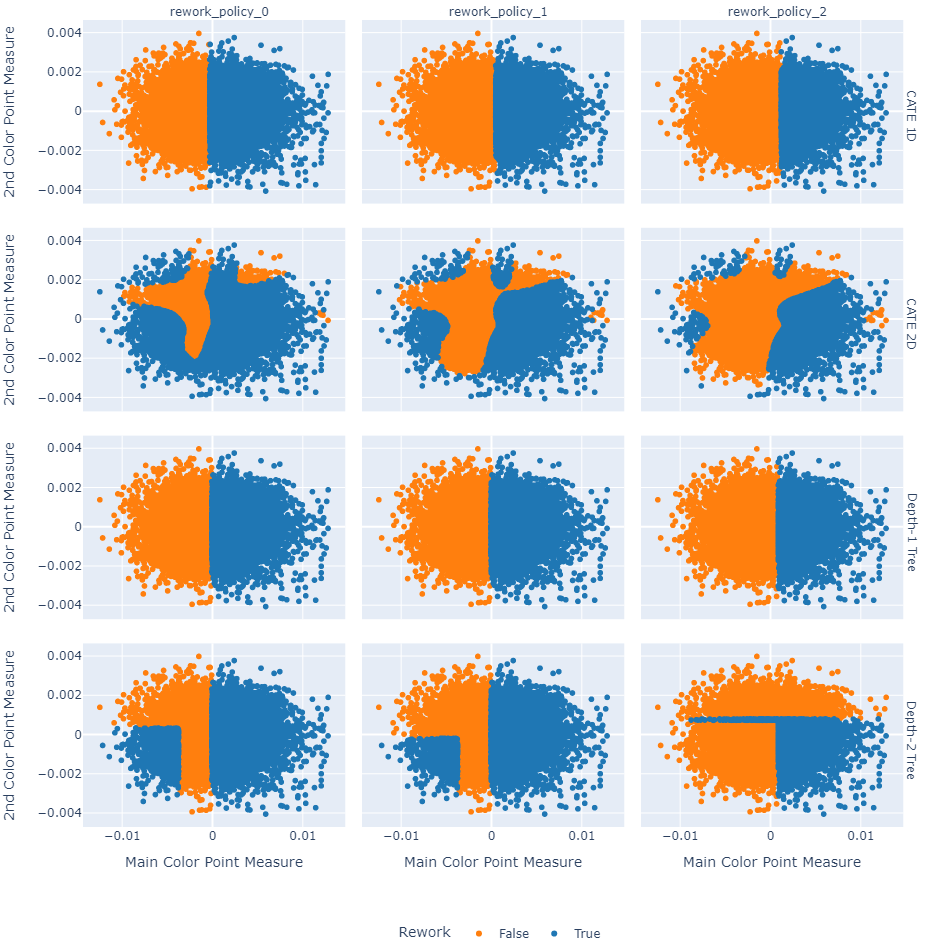}
    \caption{Comparisons of the estimated policies for product type ``T2''.}
    \label{fig:policies_l4}
\end{figure}

\begin{table}[h]
\centering
\begin{tabular}{lrrr}
\toprule
Method &  Policy 0 &  Policy 1 &  Policy 2 \\
\midrule
CATE 1D      &    0.4848 &    0.4087 &    0.3455 \\
CATE 2D      &    0.5106 &    0.3856 &    0.3127 \\
Depth-1 Tree &    0.4923 &    0.4907 &    0.3708 \\
Depth-2 Tree &    0.5624 &    0.4794 &    0.3013 \\
\bottomrule
\end{tabular}
\caption{Share of treated under the estimated policies for product type ``T2'' (Share in the observations: $0.2472$).}
\end{table}

\begin{table}[h]
\centering
\begin{tabular}{lrrr}
\toprule
Method &  Policy 0 &  Policy 1 &  Policy 2 \\
\midrule
CATE 1D      &    0.0818 &    0.0880 &    0.0961 \\
CATE 2D      &    0.0777 &    0.0950 &    0.1112 \\
Depth-1 Tree &    0.0819 &    0.0821 &    0.0951 \\
Depth-2 Tree &    0.0772 &    0.0865 &    0.1128 \\
\bottomrule
\end{tabular}
\caption{GATEs for the estimated policies for product type ``T2''. (GATE in the group of observed reworked: $0.1040$).}
\end{table}

\begin{table}[h]
\centering
\begin{tabular}{lrrr}
\toprule
Method &  Policy 0 &  Policy 1 &  Policy 2 \\
\midrule
CATE 1D      & 0.0397 & 0.0360 & 0.0332 \\
CATE 2D      & 0.0397 & 0.0366 & 0.0348 \\
Depth-1 Tree & 0.0403 & 0.0403 & 0.0353 \\
Depth-2 Tree & 0.0434 & 0.0415 & 0.0340 \\
\bottomrule
\end{tabular}
\caption{Value of the estimated policies for product type ``T2'' (Value in observed policy: $0.0036$).}
\end{table}
\newpage
