# Supplementary material for: Management Decisions in Manufacturing using Causal Machine Learning -- To Rework, or not to Rework?
Source: arXiv:2406.11308 source file (2024-06-17)
Supplement: Supplementary file 2 [file robustness_L3.tex]

\section{Robustness checks}
\label{app:rob}
\subsection{Additional Policy Learning Results}\label{app:addlearner}

In this section, we present additional results for policy learning.
The policy estimation with greedy decision trees relies on the \texttt{DecisionTreeClassifier} from \texttt{scikit-learn} \cite{scikit-learn}. We also include a weighted classification with a rbf kernel in a support vector machine. However, we caution that the theoretical bonds by \citet{athey2021} do no apply to this learning method, since they are based on bounds on the VC-dimension  of the policy class $\Pi$.

Figure \ref{fig:pol_lgbm} contains the resulting policies for the tuned ML LGBM learner as in the main analysis. We see, that the greedy tree search algorithm finds no splits along the secondary color measurement. The rbf kernel encircles little areas of color point measurements that have a higher value. The areas are very similar to the two-dimensional CATE. However, they are in an area with few observations, so the evidence from them is limited.

\begin{figure}[ht]
    \centering
    \includegraphics[width=\linewidth]{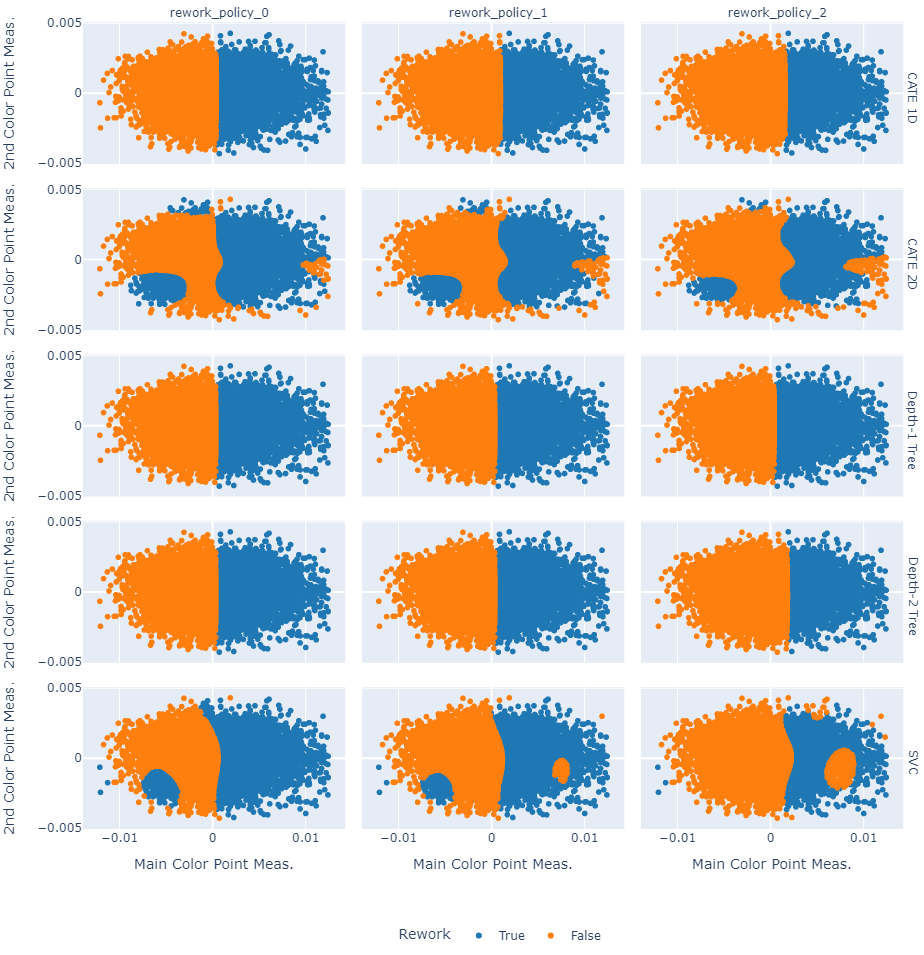}
    \caption{Comparisons of the estimated policies with additional methods.}
    \label{fig:pol_lgbm}
\end{figure}
\FloatBarrier
\subsection{DoubleML Machine Learner Comparisons}
In this section, we explore the robustness of our estimates by varying the ML method which is used to construct the estimators in Equations \ref{eq:g_0} and \ref{eq:m_0}. We compare the identical policy learning approaches as in Appendix \ref{app:addlearner}. The comparison includes results for XGBoost, random forest and linear learners. Table \ref{tab:rmse} contains the $RMSE$ of the respective ML methods in the nuisance estimation. 

\begin{table}[h]
\centering
\begin{tabular}{lrrr}
\toprule
Learner &  RMSE $m(x)$ &  RMSE $g_0(x)$ &  RMSE $g_1(x)$ \\
\midrule
Tuned LGBM    &    0.2821 &    0.8862 &    1.001 \\
XGBoost       &    0.2857 &    0.9078 &    1.043 \\
Random Forest &    0.2983 &    0.9581 &    1.077 \\
Linear Models &    0.2925 &    0.9682 &    1.083 \\
\bottomrule
\end{tabular}
\caption{RMSE for different nuisance learners.}
\label{tab:rmse}
\end{table}

Both gradient boosting frameworks achieve good predictive performance. Random forest and linear model show a slightly weaker performance. In Figures \ref{fig:pol_xg},  \ref{fig:pol_rf} and \ref{fig:pol_lin} we show the results for the policies (to allow comparisons to the learner in the main analysis in Figure \ref{fig:pol_lgbm}). The results seem to be rather robust across multiple non-linear learners, especially in the main component split. For the linear models, we see a larger deviation in the policies, which, combined with the higher nuisance $RMSE$ might indicate that linear models are not sufficient to estimate all, potentially complex, dependencies in the data.

\begin{figure}[ht]
    \centering
    \includegraphics[width=\linewidth]{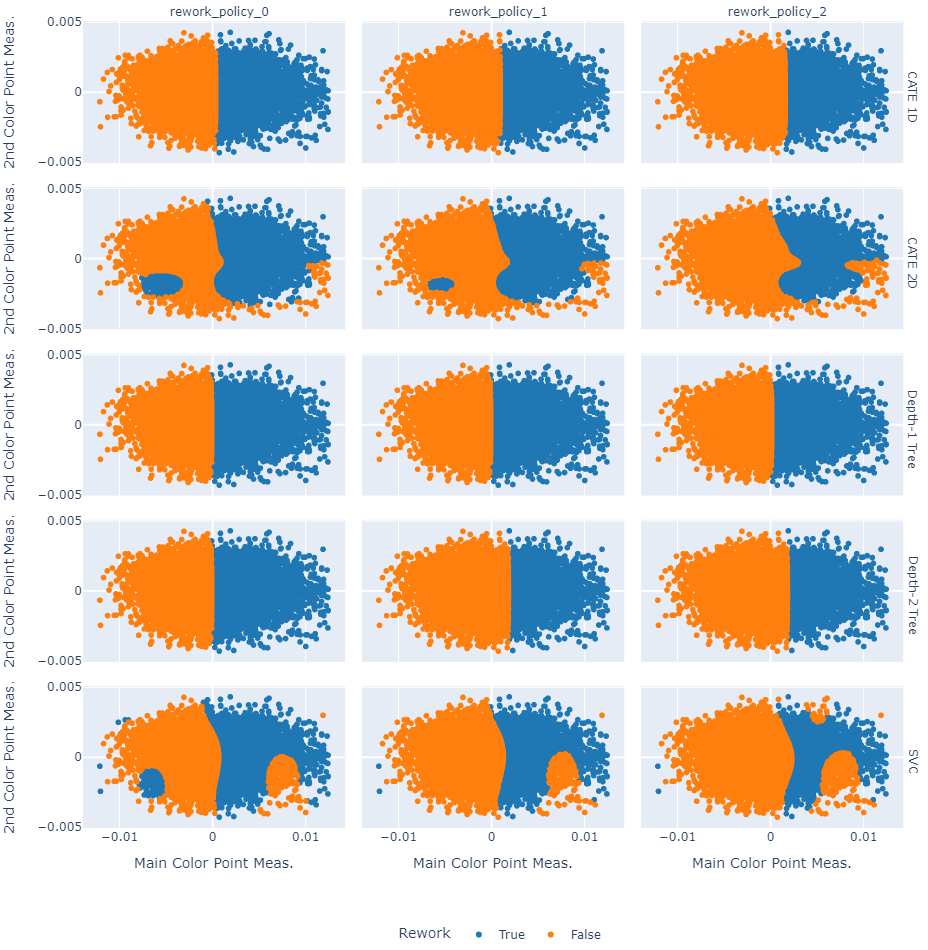}
    \caption{Comparisons of the estimated policies with the nuisance components estimated by gradient boosting implementation \texttt{xgboost}.}
    \label{fig:pol_xg}
\end{figure}

\begin{figure}[ht]
    \centering
    \includegraphics[width=\linewidth]{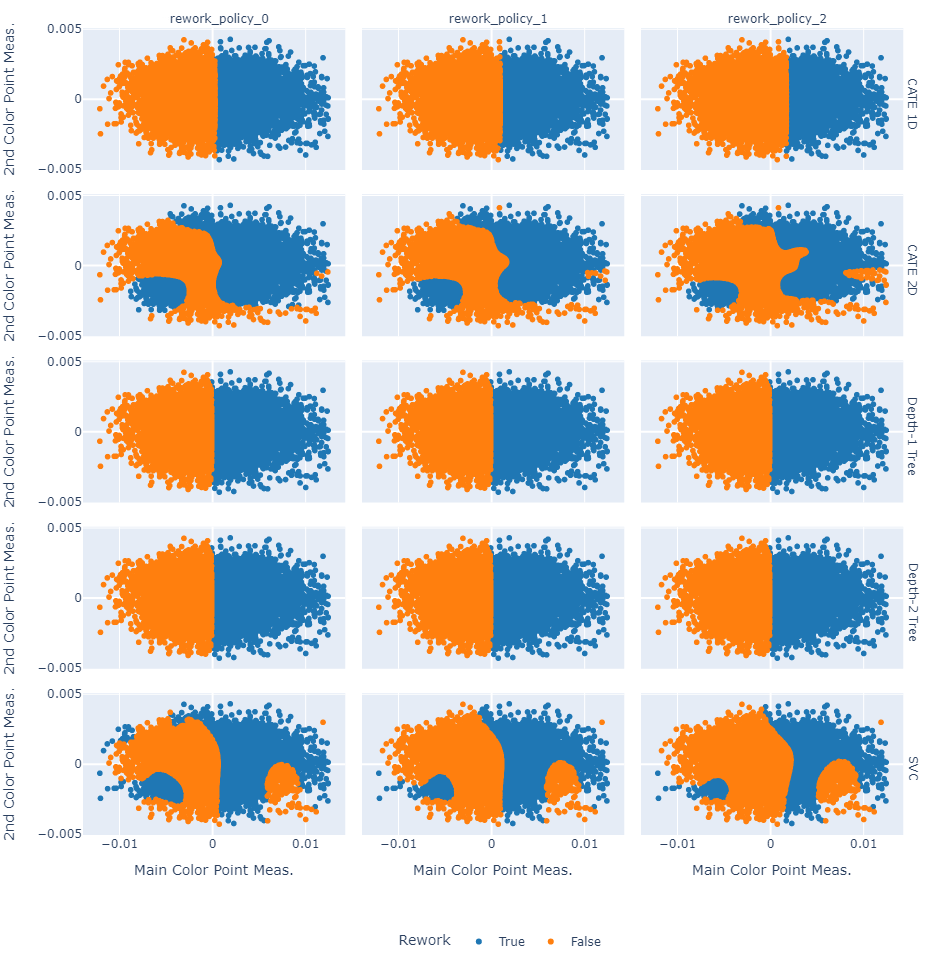}
    \caption{Comparisons of the estimated policies with the nuisance components estimated by the random forest implementation of \texttt{scikit-learn}.}
    \label{fig:pol_rf}
\end{figure}
\begin{figure}[ht]
    \centering
    \includegraphics[width=\linewidth]{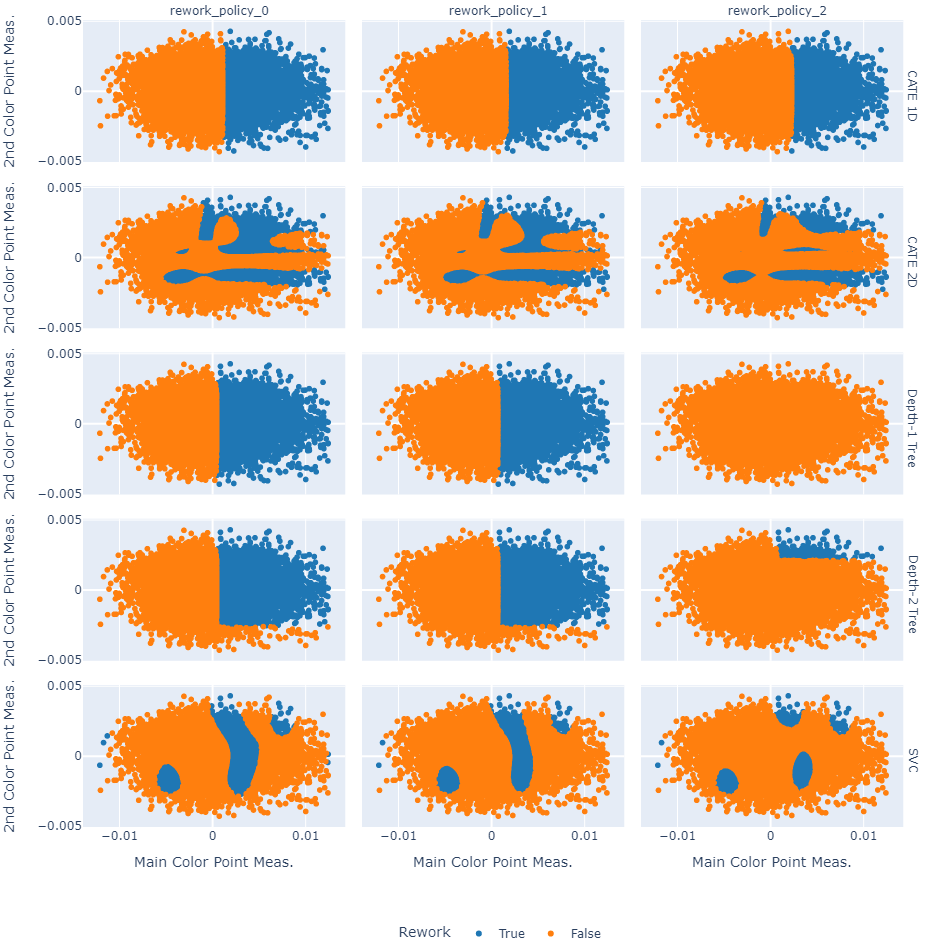}
    \caption{Comparisons of the estimated policies with the nuisance components estimated by linear models.}
    \label{fig:pol_lin}
\end{figure}
\FloatBarrier
\subsection{Policies Based on Confidence Intervals}\label{sec:confint}

As additional results, we present policies based on the conditional average treatment effect lower confidence interval. We construct a pointwise-valid confidence interval via a gaussian multiplier bootstrap as proposed in \citet{semenova2021debiased} at the level $2\alpha$. We then evaluate the lower bound to derive a rework cut-off, for which we are certain that the effect is above the desired threshold $\gamma \in \{0.01,0.03,0.05\}$ with probability $1-\alpha$. We choose $\alpha=5\%$.

Table \ref{tab:robshare} displays the share of treated under the conservative policies. We see, that compared to Table \ref{tab:policies}, less chip lots are assigned to be reworked. 

\begin{table}
\centering
\begin{tabular}{lrrr}
\toprule
Method &  Policy 0 &  Policy 1 &  Policy 2 \\
\midrule
CATE 1D &    0.3446 &    0.2754 &    0.2067 \\
CATE 2D &    0.2152 &    0.0852 &    0.0459 \\
\bottomrule
\end{tabular}
\caption{Share of treated chip lots under the conservative policies.}
\label{tab:robshare}
\end{table}

Unsurprisingly, this leads to an increase of GATE (Table \ref{tab:robgate}) in the group of treated, compared to Table \ref{tab:gate}.

\begin{table}
\centering
\begin{tabular}{lrrr}
\toprule
Method &  Policy 0 &  Policy 1 &  Policy 2 \\
\midrule
CATE 1D &    0.0758 &    0.0862 &    0.0967 \\
CATE 2D &    0.0797 &    0.0950 &    0.1328 \\
\bottomrule
\end{tabular}
\caption{Grouped average treatment effect for the group of treated chip lots under the conservative policies.}
\label{tab:robgate}
\end{table}

In the case of the one-dimensional CATE, we believe this is a possibility to make the cut-off even more conservative and still increase overall yield. In the case of the two-dimensional CATE, we are careful in interpretation, as using the confidence interval might overfit to a large extend on small areas with little observations but a potentially high value. The values of these policies are displayed in Table \ref{tab:robvalue} (in comparison to Table \ref{tab:value}).

\begin{table}
\centering
\begin{tabular}{lrrr}
\toprule
Method &      0 &      1 &      2 \\
\midrule
CATE 1D & 0.0261 & 0.0237 & 0.0200 \\
CATE 2D & 0.0171 & 0.0081 & 0.0061 \\
\bottomrule
\end{tabular}
\caption{Value of the conservative CATE policies.}
\label{tab:robvalue}
\end{table}

Additionally, we illustrate in Figure \ref{fig:full_cate} the influence of the little overlap outside the interval $C_m \in [-0.005,0.005]$. While the CATE is approximately constant, the intervals becoming increasingly large, making the analysis more difficult due to statistical uncertainty.

\begin{figure}[ht]
\includegraphics[width=\linewidth]{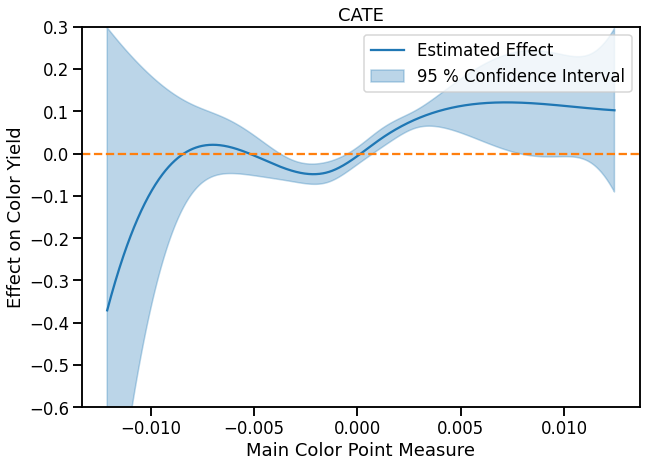}
\caption{CATE over the main color measurement for the full space of $C_m$ values.}\label{fig:full_cate}
\end{figure}
\FloatBarrier
